# Supplementary material for: Quantum fluxes at the inner horizon of a spherical charged black hole
Source: arXiv:1906.11303 ancillary file (2020-09-29)
Supplement: Supplementary file 1 [file supplemental_material.pdf]

# Supplemental Material for: Quantum fluxes at the inner horizon of a spherical charged black hole

Noa Zilberman, Adam Levi and Amos Ori

This document entails the Supplemental Material for the manuscript “Quantum fluxes at the inner horizon of a spherical charged black hole”, and is organized as follows: Section 1 demonstrates the vanishing of the flux counter-terms at the IH; Section 2 completes the derivation of the expression for  $\hat{E}_{\omega l}^H$ , as appears in Eq. (10)<sup>1</sup>; Section 3 provides an analytic computation of the constant  $\beta \equiv F_{l \rightarrow \infty}^H$ , which is subtracted as part of the regularization of the sum over  $l$  (see Eq. (11)); Section 4 serves as the Unruh counterpart of the derivation of the near-IH flux expressions, as described in the main manuscript (along with Secs. 2 and 3 of this document) for the HH state; Section 5 consists of basic details regarding the numerical parameters used in the computation, as well as the estimated numerical errors; Finally, section 6 presents the flux quantities inside a RN BH, plotted against  $r$  with closer attention on the IH vicinity, indicating a clear approach to the corresponding IH values.

## 1 The asymptotic vanishing of the flux counter-terms

As mentioned in the main manuscript, the counter-terms required for regularization of the stress-energy flux components,  $\tilde{L}_{yy}$  with  $y = u$  or  $v$ , vanish at the IH.

This should become clear from the form of  $\tilde{L}_{yy}(r)$  inside the black hole.

The  $\theta$ -splitting PMR counter-terms, obtained by processing Christensen’s counter-terms and expanding them in the splitting parameter  $\epsilon \equiv \delta\theta = \theta' - \theta$ , have the general form [8]:

$$\frac{1}{\hbar} \tilde{L}_{\mu\nu}(\epsilon) = a_{\mu\nu} \sin^{-4}(\epsilon/2) + b_{\mu\nu} \sin^{-2}(\epsilon/2) + c_{\mu\nu} \sin^{-1}(\epsilon/2) + d_{\mu\nu} \log(\sin(\epsilon/2)) + e_{\mu\nu}$$

For the two flux components, corresponding to  $\mu = \nu = y$ , we have:

$$\begin{aligned} a_{yy} &= 0 \\ b_{yy} &= f^2(r) \frac{1}{64\pi^2 r^4} \\ c_{yy} &= 0 \\ d_{yy} &= f^2(r) \frac{Q^2}{240\pi^2 r^6} \\ e_{yy} &= f^2(r) \frac{2Q^2(7 + \gamma) + Q^2 \log(r^2 \mu^2) - 9Mr}{480\pi^2 r^6} \end{aligned}$$

where  $\gamma$  is the Euler constant,  $\mu$  is an unknown scale parameter related to the ambiguity in the regularization procedure (see more in Sec. 6), and, recall,  $f(r) = (r - r_-)(r - r_+)/r^2$ . This leaves us with

$$\tilde{L}_{yy} \propto f^2(r) \propto \delta r^2$$

---

<sup>1</sup>All equation numbers appearing in this document refer to equations in the main manuscript.

where  $\delta r \equiv (r - r_-)/M$ , which clearly vanishes at the IH.

## 2 Deriving $\hat{E}_{\omega l}^H$ as appears in Eq. (10) of the main manuscript

Summing the contributions from the three “ $J$ ” terms in the expression for  $E_{\omega l m}^H(x, x')_{,uu'}$  and summing over  $m$  as indicated in the main manuscript, one would naively obtain an expression for the integrand  $\hat{E}_{\omega l}^H$  which in fact differs from that given in Eq. (10):

$$\hat{E}_{\omega l}^H = \frac{\omega \coth \tilde{\omega}}{2\pi r_-^2} \left[ (|A_{\omega l}|^2 + |B_{\omega l}|^2) + 2 \cosh^{-1} \tilde{\omega} \Re(\rho_{\omega l}^{up} A_{\omega l} B_{\omega l}) \right].$$

, the relation  $|B_{\omega l}|^2 = 1 + |A_{\omega l}|^2$ , resulting from Wronskian conservation of solutions for the radial equation (2), may be used to rewrite  $\hat{E}_{\omega l}^H$  as

$$\hat{E}_{\omega l}^H = \frac{\omega \coth \tilde{\omega}}{\pi r_-^2} \left[ |A_{\omega l}|^2 + \cosh^{-1} \tilde{\omega} \Re(\rho_{\omega l}^{up} A_{\omega l} B_{\omega l}) \right] + \frac{\omega \coth \tilde{\omega}}{2\pi r_-^2}.$$

However, the last term here is clearly  $l$ -independent, so it may be omitted by means of the so-called “blind-spot” self-cancellation phenomenon, leaving  $\hat{E}_{\omega l}^H$  as specified in Eq. (10).

In a nutshell, the subtraction of the “blind-spot” is justified by the vanishing of the generalized sum in the coincidence limit:

$$\lim_{\delta\theta \rightarrow 0} \sum_{l=0}^{\infty} (2l+1) P_l(\cos \delta\theta) = 0,$$

as proven and discussed more generally in [3].

## 3 Obtaining the large- $l$ plateau value $\beta \equiv F_{l \rightarrow \infty}$ as appears in the main manuscript

In this section, we denote  $\tilde{\omega}_{\pm} = \pi\omega/\kappa_{\pm}$  (for the sake of uniformity). However, note that  $\tilde{\omega}_+$  appearing here coincides with  $\tilde{\omega}$  appearing elsewhere, in the other sections of this document and in the main manuscript.

We wish to analytically find the plateau value (namely the large- $l$  behavior) of  $F_l^H \equiv \int_0^\infty d\omega \hat{E}_{\omega l}^H$ , where the integrand is given in Eq. (10), and quoted here for convenience:

$$\hat{E}_{\omega l}^H = \frac{\omega \coth \tilde{\omega}_+}{\pi r_-^2} \left[ |A_{\omega l}|^2 + \cosh^{-1} \tilde{\omega}_+ \Re(\rho_{\omega l}^{up} A_{\omega l} B_{\omega l}) \right].$$

Taking the large- $l$  limit of  $F_l^H$  yields a constant value (denoted by  $\beta$ ), which may be subtracted from  $F_l^H$  while summing, hence regularizing the sum (this  $l$ -independent term is a “blind-spot”, as described already in Sec. 2). Our goal here is to analytically compute this constant.

We begin by considering the large- $l$  limit of the integrand, and then perform the integration over  $\omega$ . We shall use the large- $l$  expressions for  $A_{\omega l}$ ,  $B_{\omega l}$  and  $\rho_{\omega l}$ , as derived in Ref. [1] (and are given in Eqs. (5.22), (5.21) and (3.17) therein, respectively). For the first term appearing in Eq. (10) we find, utilizing  $\Gamma$ -function identities:

$$\lim_{l \rightarrow \infty} |A_{\omega l}|^2 = \frac{\sinh^2[(\tilde{\omega}_+ - \tilde{\omega}_-)/2]}{\sinh \tilde{\omega}_+ \sinh \tilde{\omega}_-}.$$

Similarly, the second term involving the product of all three quantities yields:

$$\lim_{l \rightarrow \infty} \rho_{\omega l}^{up} A_{\omega l} B_{\omega l} = \frac{\sinh[(\tilde{\omega}_+ - \tilde{\omega}_-)/2] \sinh[(\tilde{\omega}_+ + \tilde{\omega}_-)/2]}{\sinh \tilde{\omega}_+ \sinh \tilde{\omega}_-}.$$

Altogether, these combine to give the large- $l$  limit of the integrand:

$$\hat{E}_{\omega(l \rightarrow \infty)}^H = \frac{\omega}{2\pi r_-^2} (\coth \tilde{\omega}_- - \coth \tilde{\omega}_+).$$

Finally, integrating over  $\omega$ , the large- $l$  plateau value is obtained: <sup>2</sup>

$$\beta = \frac{1}{24\pi r_-^2} (\kappa_-^2 - \kappa_+^2).$$

Two remarks are in order: (i) The large- $l$  behavior computed here exclusively for the HH near-IH flux expression is, in fact, shared by all three flux quantities (that is, by  $\langle T_{uu} \rangle_{ren}^U$  and  $\langle T_{vv} \rangle_{ren}^U$  as well). To see this, note that the difference in the corresponding  $F_l$  series is  $\Delta F_{l(yy)}^U \equiv \int_0^\infty d\omega \Delta \hat{E}_{\omega l(yy)}^U$ , where  $\Delta \hat{E}_{\omega l(yy)}^U \propto |\tau_{\omega l}^{up}|^2$  (see Eq. (13), or the next section of this document).  $|\tau_{\omega l}^{up}|^2$  clearly vanishes in the large- $l$  limit, while the other factors in the product converge, leaving a vanishing large- $l$  contribution; and (ii) It actually proves more efficient, in the numerical implementation, to subtract the large- $l$  behavior already at the integrand level, before performing the  $\omega$ -integration that yields the  $F_l$  series. With this subtraction, the integrand decays rapidly with increasing  $l$  (per given  $\omega$ ), leading to reduced numerical error.

## 4 Obtaining the near-IH flux expressions for the Unruh state

In the main manuscript, the near-IH flux expressions were explicitly derived for the HH state. Here, we shall carry the analogous treatment for the Unruh state.

We begin with Eq. (6), where the mode contributions  $E_{\omega lm}(x, x')$  in the Unruh state inside a RN BH are given by:

$$E_{\omega lm}^U(x, x') = E_{\omega lm}^H(x, x') + (1 - \coth \tilde{\omega}) |\tau_{\omega l}^{up}|^2 J^R$$

where, recall,  $J^R = \{f_{\omega lm}^R(x), f_{\omega lm}^{R*}(x')\}$  (cf. Eq. (4.2) in Ref. [2]). As in the HH case, we may write

$$\langle T_{yy} \rangle_{ren}^U(x) = \frac{\hbar}{2} \lim_{x' \rightarrow x} \sum_{l,m} \int_0^\infty d\omega E_{\omega lm}^U(x, x')_{,yy'}.$$

Aiming for both flux components  $\langle T_{uu}^- \rangle_{ren}^U$  and  $\langle T_{vv}^- \rangle_{ren}^U$ , we should evaluate  $J_{,yy'}^R$ , for both  $y = u$  and  $y = v$  within the near-IH asymptotic approximation. The  $y = u$  case has already been computed in the main manuscript, resulting in Eq. (8). The  $y = v$  case may be treated equivalently, yielding

$$J_{,vv'}^R \rightarrow \frac{|\omega|}{4\pi r_-^2} \{Y_{lm}(\theta, \varphi), Y_{lm}^*(\theta', \varphi)\} |B_{\omega l}|^2.$$

Utilizing the Wronskian relation  $|A_{\omega l}|^2 + 1 = |B_{\omega l}|^2$ , we may compactly write:

$$J_{,yy'}^R \rightarrow \frac{|\omega|}{4\pi r_-^2} \{Y_{lm}(\theta, \varphi), Y_{lm}^*(\theta', \varphi)\} (|A_{\omega l}|^2 + \delta_y^v).$$

---

<sup>2</sup>This derivation actually entails interchanging the order of the  $\omega$ -integration and the large- $l$  limit. We are currently unable to rigorously prove the validity of this interchange. Nevertheless, this analytically-computed  $\beta$  matches the numerical large- $l$  plateau value extremely well.

Note that here, just as in the HH state, the expressions are independent of  $r_*$ , as the oscillatory terms originating from the asymptotic approximation for  $\tilde{f}_{\omega l}^R$  (as given in Eq. (7)) cancel out. Summing over  $m$ , using the spherical harmonics identity

$$\sum_{m=-l}^l Y_{lm}(\theta, \varphi) Y_{lm}^*(\theta + \delta\theta, \varphi) = \frac{2l+1}{4\pi} P_l(\cos \delta\theta) ,$$

one obtains

$$\langle T_{yy} \rangle_{ren}^U = \langle T_{yy} \rangle_{ren}^H + \hbar \lim_{\delta\theta \rightarrow 0} \sum_{l=0}^{\infty} \frac{2l+1}{8\pi} P_l(\cos \delta\theta) \Delta F_{l(yy)}^U ,$$

with  $\Delta F_{l(yy)}^U \equiv \int_0^\infty d\omega \Delta \hat{E}_{\omega l(yy)}^U$ , where

$$\Delta \hat{E}_{\omega l(yy)}^U \equiv \hat{E}_{\omega l(yy)}^U - \hat{E}_{\omega l}^H = \frac{\omega}{2\pi r_-^2} (1 - \coth \tilde{\omega}) |\tau_{\omega l}^{up}|^2 \left( |A_{\omega l}|^2 + \delta_y^v \right) .$$

The sequence  $\Delta F_{l(yy)}^U$  decays to 0 at large  $l$ , as mentioned at the end of Sec. 3. In general, one finds that all “blind-spots” occurring in the HH case are shared by the Unruh case, implying the regularity of their difference at the IH. We may thus safely take the coincidence limit (that is,  $\delta\theta \rightarrow 0$ ) and obtain the final expression for the near-IH fluxes in the Unruh state:

$$\langle T_{yy}^- \rangle_{ren}^U = \langle T_{yy}^- \rangle_{ren}^H + \hbar \sum_{l=0}^{\infty} \frac{2l+1}{8\pi} \Delta F_{l(yy)}^U .$$

By this we have recovered Eqs. (12,13).

We point out that an analogous expression may be derived at the EH (approached from  $r < r_+$ ). Hereafter, we shall denote this limit by a superscript “+”. The asymptotic form of the mode functions at the EH requires taking  $A_{\omega l}^+ = 0$  and  $B_{\omega l}^+ = 1$  (recall from Eq. (4) that we assume an incoming wave,  $\psi_{\omega l} \cong e^{-i\omega r_*}$ ). This yields  $\langle T_{uu}^+ \rangle_{ren} = 0$  in both quantum states, as seen in (the EH counterparts of) Eqs. (10) and (13). This vanishing of  $\langle T_{uu}^+ \rangle_{ren}$  also follows from the demand for regularity at the EH (as may be seen by transforming to a Kruskal-like coordinate at the EH,  $U^+ = e^{\kappa+u}$ ).

Another remark, already referred to in the main manuscript, is worth making. For spherically-symmetric static BH backgrounds (like Schwarzschild or RN), energy-momentum conservation implies that in any quantum state which is spherically symmetric and  $t$ -translation invariant (like the Unruh and HH states), the quantity  $4\pi r^2 (\langle T_{uu}(x) \rangle_{ren} - \langle T_{vv}(x) \rangle_{ren})$  must be *constant* throughout spacetime. In the HH state, this constant trivially vanishes. In the Unruh state, it should coincide with the *Hawking outflux*. Using the above results for  $\langle T_{yy}^- \rangle_{ren}^U$ , we may compute this quantity directly at the IH:

$$4\pi r_-^2 \left( \langle T_{uu}^- \rangle_{ren}^U - \langle T_{vv}^- \rangle_{ren}^U \right) = \hbar \sum_{l=0}^{\infty} \frac{2l+1}{4\pi} \int_0^\infty d\omega \omega (\coth \tilde{\omega} - 1) |\tau_{\omega l}^{up}|^2 .$$

This indeed reproduces the well-known expression for the luminosity of an evaporating BH. (See, for example, Eq. (136) in Ref. [6] or Eq. (6.20) in Ref. [7] for the Schwarzschild case. The only modification needed is replacing the Schwarzschild  $\kappa$  parameter by the RN  $\kappa_+$ .)

## 5 Numerical parameters

Throughout the range  $0.1 \leq Q/M \leq 0.9$ , we inspected  $Q/M$  values in steps of 0.05. Then, in the domain of larger  $Q/M$ , we halved the distance to extremality in each step, going from 0.9 up to  $1 - 0.1 \times 2^{-15}$ . The *sign-flip* region is a domain centered at around  $Q/M \sim 0.97$ , in which we further refined the data points so that the critical values

of transition,  $q_y^H$ ,  $q_u^U$  and  $q_v^U$ , could be extracted to the desired precision.

For each  $Q/M$  value we computed  $\omega l$  modes in adequate  $l$  and  $\omega$  ranges. We typically included  $l$  values whose relative contribution to the sum over  $l$  is of at least  $10^{-6}$ . For each  $l$  we terminated the numerical  $\omega$  integration when the integrand  $\hat{E}_{\omega l}$  has entered deep into the expected large- $\omega$  decay, in which it behaves like  $\omega$  times a decaying exponent (due to the exponential decay of the dominant  $|A_{\omega l}|^2$  term at large  $\omega$ , combined with the  $\omega$  factor present in the integrand in Eqs. (10) and (13)). From this range of large  $\omega$  we extracted the relevant parameters, which allowed us to analytically extend the integration over  $\omega$  all the way to  $\infty$ . In the very near-extremal domain, characterized by the parameter  $\Delta \equiv \sqrt{1 - (Q/M)^2}$  being exceedingly small, it suffices to include the  $l = 0$  contribution (it turns out, both analytically and numerically, that  $F_l - \beta$  decays steeply with  $l$  as  $Q/M$  increases towards 1. We intend to further elaborate on this point in a future paper [5]). In that domain, guided by analytical insights, we chose an  $\omega$  range which suitably scales with  $\Delta$  (typically,  $\omega \in [10^{-2}M^{-1}\Delta, 10M^{-1}\Delta]$ ).

As in any numerical work, errors are inevitable. The sources of numerical error were identified and estimated throughout the  $Q/M$  range. We estimate our *relative* numerical error to be bounded from above by  $10^{-3}$  in the entire  $Q/M$  range — except for the very narrow domains of sign-flip for each of the three flux quantities, given by (say)  $Q/M \in [q_y^{H,U} - 10^{-4}, q_y^{H,U} + 10^{-4}]$ , where  $q_y^{H,U}$  refers respectively to  $q_y^H$ ,  $q_u^U$  or  $q_v^U$ , the  $Q/M$  values of sign-flip (see the main manuscript for concrete values). The error in these narrow domains has to be expressed differently, of course, since the relative error diverges by definition as the fluxes cross the zero line. Hence, here we present the *absolute* error rather than the relative one, finding a shared upper bound of  $10^{-10}\hbar M^{-4}$ . A convenient way to translate this absolute error into a dimensionless one is by inspecting the amount by which such an error in the fluxes would modify  $q_y^{H,U}$ , the  $Q/M$  values of sign change. (This translation of the error from “vertical” to “horizontal” terms involves a division by the local slope of the flux curves, namely, the rate of change of the fluxes with  $Q/M$ ). We find that this reflected error in  $q_y^{H,U}$  is bounded from above by  $10^{-7}$ .

The three sign-flip values  $q_y^{H,U}$  are found by interpolating the fluxes between the discrete  $Q/M$  values where the fluxes were actually computed. When evaluating the error in the numerically-computed  $q_y^{H,U}$  values, in addition to the aforementioned  $\lesssim 10^{-7}$  uncertainty emerging from the errors in the fluxes, there also is an inevitable interpolation error. We estimate this interpolation error to be  $\lesssim 10^{-6}$ , hence it dominates the overall estimated error in the evaluation of  $q_y^{H,U}$ . (Thus, in the values specified in the main manuscript for  $q_y^{H,U}$ , all four digits are significant.)

## 6 Fluxes on approaching the IH

The flux components,  $\langle T_{uu} \rangle_{ren}$  and  $\langle T_{vv} \rangle_{ren}$ , on a fixed RN background metric and at both quantum states (Unruh and HH), are functions of  $r$  only. In the paper, we focused specifically on the *IH values* of these fluxes (namely their values at  $r = r_-$ ). In practice, this computation was done by taking the  $r \rightarrow r_-$  limit already at the integrand in Eq. (6). Note, however, that this procedure involves interchanging the limit  $r \rightarrow r_-$  with the integration over  $\omega$  and the summation over  $l, m$  (and also with the coincidence limit  $x' \rightarrow x$ ). One may be concerned about the mathematical validity of these interchanges, which we are currently unable to rigorously prove.

To bridge this gap in our analysis, we computed the renormalized flux quantities  $\langle T_{uu} \rangle_{ren}(r)$  and  $\langle T_{vv} \rangle_{ren}(r)$  away from the IH and observed their  $r \rightarrow r_-$  limit, examining whether this limit matches the corresponding IH values as derived in the paper. For this examination, we chose two  $Q/M$  values - one which admits positive flux quantities at the IH ( $Q/M = 0.8$ ), and the other admitting negative flux quantities at the IH ( $Q/M = 0.975$ ). Fig. 1 displays the results of these computations, in which the renormalized fluxes (in both quantum states) are plotted against  $\delta r = (r - r_-)/M$  in the IH vicinity.

The relative numerical error in the results presented in Fig. 1 is estimated to be bound by  $\lesssim 0.2\%$  for both  $Q/M$  values.

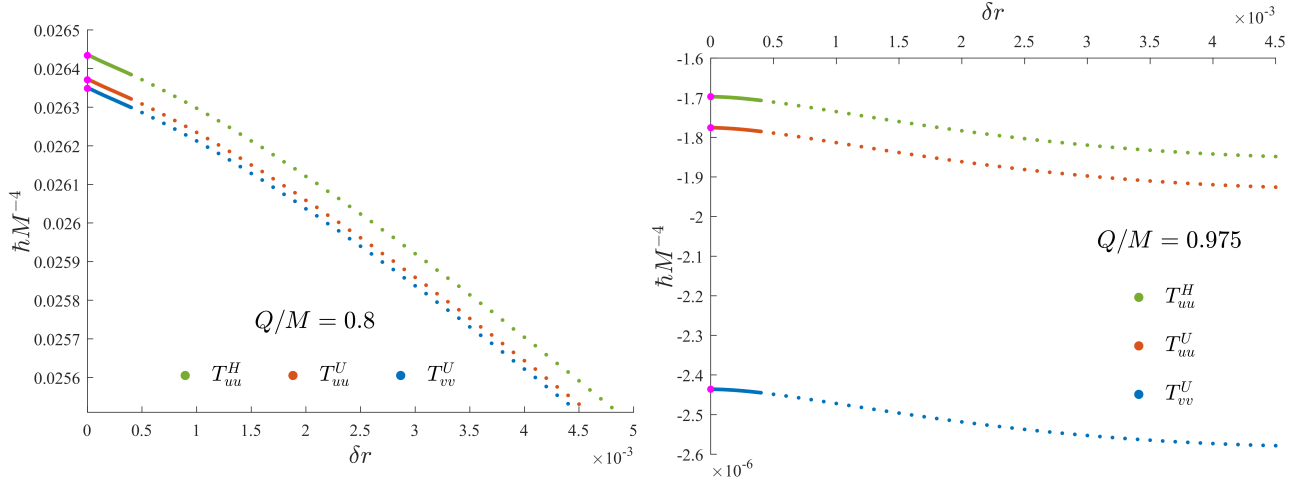

Figure 1:  $\langle T_{yy} \rangle_{ren}$  (namely  $\langle T_{uu} \rangle_{ren}^U$ ,  $\langle T_{vv} \rangle_{ren}^U$ , and  $\langle T_{uu} \rangle_{ren}^H = \langle T_{vv} \rangle_{ren}^H$ ) as a function of  $\delta r$ . The pink points at  $\delta r = 0$  are the corresponding values at the IH, presented in the main manuscript. On the left: results for a RN BH with  $Q/M = 0.8$ . On the right: results for a RN BH with  $Q/M = 0.975$ .

Here, the flux quantities were computed via the general- $r$  expression derived from the generalization of Eq. (5) for an arbitrary spacetime point (where the counter-terms no longer vanish):

$$\langle T_{yy} \rangle_{ren}(x) = \lim_{x' \rightarrow x} \left( \frac{\hbar}{2} G^{(1)}(x, x')_{,yy'} - \tilde{L}_{yy}(x, x') \right)$$

which was further treated according to the standard  $\theta$ -splitting variant of the PMR method [3, 4, 8]. The resulting expression is clearly more complicated than the one obtained at the IH (Eqs. (10-13)), but this doesn't pose any serious difficulty in performing the calculation.

Inspecting Fig. 1, one may observe that the IH value derived in the main manuscript (whose computation went through the aforementioned exchange of limits), is indeed approached as the  $r \rightarrow r_-$  limit of our general- $r$  results. Quantitatively speaking, the relative difference between the IH value and the numerical values extrapolated to  $r = r_-$  is  $\lesssim 2 \times 10^{-5}$  for  $Q/M = 0.8$  and  $\lesssim 1 \times 10^{-5}$  for  $Q/M = 0.975$ <sup>3</sup>, fully consistent with the anticipated numerical and extrapolation errors. This settles (at least on the numerical level) the issue of the exchange of limits, and corroborates the IH results presented in the main manuscript.

With this, we have completed our main goal. However, since we have developed the tools needed for computation of the flux quantities at a general  $r$  value inside the BH, it is worth utilizing them to further examine the fluxes in the entire BH interior domain between the EH and the IH. So far we only got initial results (for instance, we only looked at two  $Q/M$  values), but these results are still worth presenting.

Regularity of the metric at the EH combined with basic properties of the quantum states dictate  $\langle T_{uu} \rangle_{ren}^U = \langle T_{uu} \rangle_{ren}^H = \langle T_{vv} \rangle_{ren}^H = 0$  at the EH, as well as  $\langle T_{vv} \rangle_{ren}^U < 0$  there. The flux components then evolve as the field propagates inwards, changing with  $r$  as it varies from  $r_+$  to  $r_-$ . Note, for example, that while  $\langle T_{vv} \rangle_{ren}^U$  starts as negative at the EH, we found it can have either sign (or vanish) at the IH. The flux quantities thus have a non-trivial behavior between the horizons, which may be explored numerically.

It is worth mentioning a particular subtlety that arises in the computation of the flux quantities at a general  $r$  value. The term  $\log(r^2 \mu^2)$  appearing in the finite counter-term  $e_{yy}$  in Sec. 1 contains the unknown parameter  $\mu$ <sup>4</sup>.

<sup>3</sup>In both cases, the innermost  $\delta r$  value taken into account is  $10^{-6}$ .

<sup>4</sup>This ambiguous logarithmic term only exists for non-vacuum background metrics.

It is useful to re-express this term as:

$$\log(r^2\mu^2) = \log(r^2/M^2) + 2\log(M\mu) ,$$

and we now concentrate on the term  $\log(M\mu)$ .

While for a massive field some authors take  $\mu$  to be related to the field's mass, in the present case of a massless field this association is meaningless. Since the natural mass scale in the context of semiclassical gravity is the Planck mass  $m_p$ , we may assume  $\mu$  to be of the order of  $1/m_p$ .

Remarkably, this  $M$ -dependent term breaks the otherwise-universal nature of the renormalized stress energy, that is, invariance of  $M^4 \langle T_{\alpha\beta} \rangle$  under scaling in which one fixes  $Q/M$  (as well as  $r/M$ ). Since  $e_{yy}$  vanishes at the IH, this term didn't affect the results there, which are indeed universal in the mentioned sense. However, at a general  $r$  this term adds the finite contribution  $-\hbar \log(M\mu) f^2(r) Q^2/240\pi^2 r^6$  to all flux components  $\langle T_{yy} \rangle_{ren}$ .

Since this finite ambiguous logarithmic term vanishes at the IH like  $f^2 \propto (r - r_-)^2$ , it has absolutely no effect on our main goal of validating our results at the IH. For this reason, in Fig. 1, which was intended for that purpose, the plots were shown for the simplest choice  $M = 1/\mu$ , so that the  $\log(M\mu)$  term vanishes. However, in our second goal of portraying the fluxes between the two horizons for astrophysical BHs, this term does have a notable effect and should be taken into account. Clearly, in this context the choice  $M = 1/\mu$  is highly unrealistic (as astrophysical BH masses are larger than the Planck mass by some 40-50 orders of magnitude). For this reason, in Fig. 2 we show the fluxes between the two horizons for two typical astrophysical mass values, corresponding to stellar and super-massive BHs (and also for the fiducial value  $M = 1/\mu$ ).

Note that in the scale used in Fig. 2 (dictated by the range  $r_- \leq r \leq r_+$  and by the astrophysical masses) the tiny differences between the three flux quantities are barely distinguishable (see figure caption).

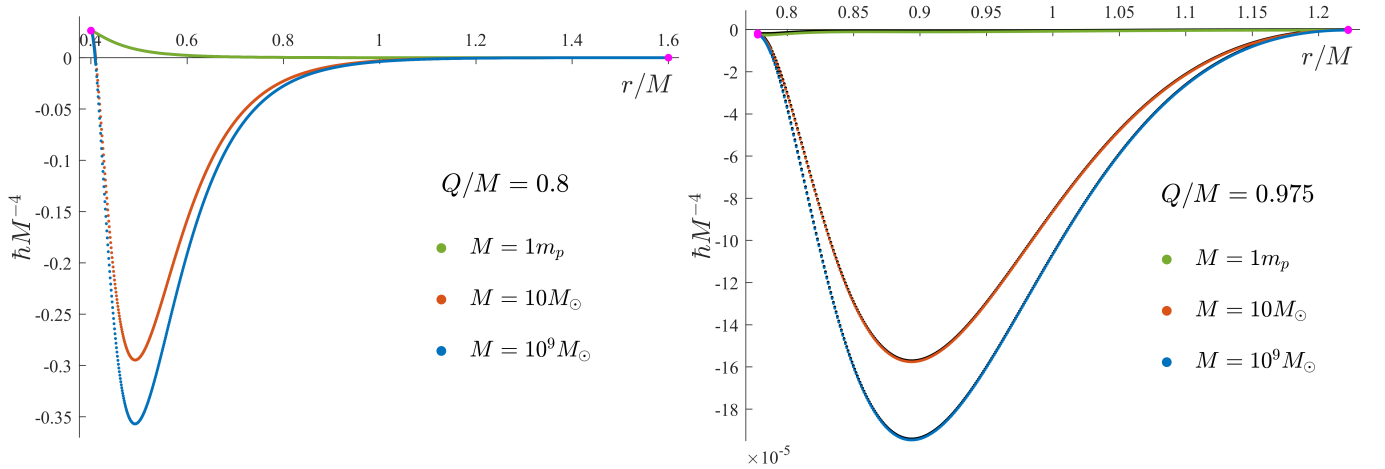

Figure 2: The flux quantities as a function of  $r$ , for BHs of mass  $M = m_p$ ,  $M = 10M_\odot$  (stellar BH) and  $M = 10^9M_\odot$  (super-massive BH), where  $\mu$  was taken to be  $1/m_p$ . The colorful markers in each  $M$  value denote  $\langle T_{vv} \rangle_{ren}^U$ , while the black markers (placed underneath and hence hardly seen) denote  $\langle T_{uu} \rangle_{ren}^U$  and  $\langle T_{uu} \rangle_{ren}^H$ . The two latter curves are indistinguishable from one another, as well as barely distinguishable from  $\langle T_{vv} \rangle_{ren}^U$ , at this scale. (When translated to a general  $\mu$ , the green, red and blue markers respectively correspond to  $M\mu = 1$ ,  $M\mu \cong 9.14 \times 10^{38}$ , and  $M\mu \cong 9.14 \times 10^{46}$ .) The pink points correspond to the horizons, the points at  $r = r_-$  being the IH values (obtained in the main paper) and the points at  $r = r_+$  being 0 for  $\langle T_{uu} \rangle_{ren}$  in both quantum states, and the Hawking outflux divided by  $-4\pi r_+^2$  for  $\langle T_{vv} \rangle_{ren}^U$ . (Although, at the scale of the figure, the deviation of this quantity from zero is too small to be noticed). On the left: results for RN BHs with  $Q/M = 0.8$ . On the right: results for RN BHs with  $Q/M = 0.975$ .

In the results presented in Fig. 2, we estimate our absolute numerical errors in the entire  $r_- < r < r_+$  range to be bound by  $\lesssim 8 \times 10^{-5} \hbar M^{-4}$  and  $\lesssim 10^{-7} \hbar M^{-4}$  for  $Q/M = 0.8$  and  $Q/M = 0.975$ , respectively.<sup>5</sup>

## References

- [1] O. Sela, *Quantum effects near the Cauchy horizon of a Reissner-Nordstrom black hole*, Phys. Rev. D. **98**, 024025 (2018).
- [2] A. Lanir, A. Levi, A. Ori and O. Sela, *Two-point function of a quantum scalar field in the interior region of a Reissner-Nordstrom black hole*, Phys. Rev. D. **97**, 024033 (2018).
- [3] A. Levi and A. Ori, *Mode-sum regularization of  $\langle \phi^2 \rangle$  in the angular-splitting method*, Phys. Rev. D. **94**, 044054 (2016).
- [4] A. Levi and A. Ori, *Versatile Method for Renormalized Stress-Energy Computation in Black-Hole Spacetimes*, Phys. Rev. Lett. **117**, 231101 (2016).
- [5] N. Zilberman et al., *Quantum fluxes at the inner horizon of a nearly extremal spherical charged black hole*, in preparation.
- [6] B. S. DeWitt, *Quantum field theory in curved spacetime*, Phys. Rep. C. **19**, 295 (1975).
- [7] S. M. Christensen and S. A. Fulling, *Trace anomalies and the Hawking effect*, Phys. Rev. D. **15**, 2088 (1977).
- [8] A. Levi, *Stress-energy tensor mode-sum regularization in spherically symmetric backgrounds*, in preparation.

---

<sup>5</sup>Given the fact that zero crossing occurs in both figures, in order to express this numerical error in a relative manner, we may compare it to the peak of the corresponding  $M = 10^9 M_\odot$  plot (which gives, essentially, the scale of the corresponding figure). This yields relative errors smaller than 0.05% for both  $Q/M$  values.
